# Supplementary material for: Does Vec2Text Pose a New Corpus Poisoning Threat?
Source: arXiv:2410.06628 source file (2024-10-09)
Supplement: Supplementary file 1 [file appendix.tex]

\section{APPENDIX?}
